# Supplementary material for: Retrospective Search for Strongly Lensed Supernovae in the DESI Legacy Imaging Surveys
Source: arXiv:2301.03578 source file (2023-03-31)
Supplement: Supplementary file 1 [file appendix_old.tex]

\section{Strong Gravitational Lensing Formalism}

Strong gravitational lensing occurs when a massive object (e.g., a galaxy or galaxy cluster), is almost aligned with a distant object, and the gravity of the foreground object (lens) bends the light from the background object (source).  The distances to the source ($D_s$), to the lens ($D_d$), and between the source and lens ($D_{ds}$) are all much larger than the scale of the lens.  It is therefore convenient to define the plane perpendicular to the observer that contains the lens as the lens plane, where ``light bending" (or lensing) occurs. 
\begin{figure}[H]
\begin{center}
\includegraphics[width=170mm]{data_figures/lensing_dia.PNG}
\caption{A simple schematic of strong gravitational lensing.  O is the observer, S is the location of the source, and I is the lensed image location.  This diagram defines relevant angular and distance parameters: $\alpha, \beta, \theta, D_{ds}, D_{d},$ and $D_{s}$.}
\end{center}
\end{figure}

From Figure 1, it is clear that:
\begin{equation}
    \vec{\beta} = \vec{\theta} - \vec{\alpha}(\vec{\theta})
\end{equation}
This is known as the lens equation, where $\vec{\beta}$, $\vec{\theta}$, and  $\vec{\alpha}(\vec{\theta})$  represent the source position, the image location, and the deflection angle, respectively.

Additionally, since we assume lensing occurs solely on the lens plane, we can collapse the gravitational potential of the lensing from a 3D quantity to a 2D potential along the line of sight:
\begin{equation}
    \psi(\vec{\theta}) = \frac{2D_{ds}}{c^2D_dD_s}\int \Phi(D_d\vec{\theta}, z)dz,
\end{equation}
where $\Phi$ is the Newtonian potential of the lens.  We can deduce that the gradient of $\psi$ with respect to $\theta$ results in the deflection angle, $\vec{\alpha}(\vec{\theta})$:
\begin{equation}
    \vec{\nabla}_\theta\psi = \frac{2D_{ds}}{c^2D_s}\int \vec{\nabla}_\perp \Phi dz = \vec{\alpha}(\vec{\theta})
\end{equation}
In order to calculate the time delay of the images, we have to find both the geometric and gravitational time delays.  The geometric time delay is caused by the curved path light now follows due to lensing, and can be calculated as follows (e.g., \_\_\_):
\begin{equation}
    \Delta t_{geom}(\vec{\theta}) = (1+z_d)\frac{D_{\Delta t}}{2c}(\vec{\alpha}(\vec{\theta}))^2=(1+z_d)\frac{D_{\Delta t}}{2c}(\vec{\theta}-\vec{\beta})^2,
\end{equation}
where $D_{\Delta t} \equiv \frac{D_dD_s}{D_{ds}}$ (also  referred to as the time delay distance).

The gravitational (Shapiro) time delay is caused by the gravitational time dilation due to the lensing potential.  This can be computed by multiplying the time delay distance with the integral over the Newtonian potential of the lensing system (\citealp{shapiro}), resulting in:
\begin{equation}
    \Delta t_{grav}(\vec{\theta}) = -(1+z_d)\frac{\dTD}{c}\psi(\vec{\theta})
\end{equation}
The total time delay is the sum of the geometric and gravitational components:
% \begin{equation}
%     \Delta t(\vec{\theta}) = \Delta t_{geom}(\vec{\theta}) + \Delta t_{grav}(\vec{\theta})
% \end{equation}
\begin{equation}
    \Delta t(\vec{\theta}) = \frac{(1+z_d)}{c}\dTD\left[ \frac{1}{2}(\vec{\theta}-\vec{\beta})^2 - \psi(\vec{\theta}) \right],
\end{equation}
where $D_d,D_{s},D_{ds}$ are angular diameter distances.  Each distance is linearly related to $\frac{1}{H_0}$ (\citealp{e10}). Therefore: 
\begin{equation}
    {\Delta t(\vec{\theta})  \propto \frac{1}{H_0}}
\end{equation}


The magnification, $\mu$, of a lensed image is by definition the ratio between the differential image area and the corresponding differential source area, and is a function of $\theta$.  Therefore the magnification can be calculated from the negative Jacobian matrix of the lensing potential:

\begin{equation}
    A = -\begin{pmatrix}
    \psi_{11} & \psi_{12} \\
    \psi_{21} & \psi_{22} 
    \end{pmatrix}, 
    \psi_{ij}=\frac{\partial^2\psi}{\partial\theta_i\theta_j}
\end{equation}
\begin{equation}
    \mu=(\det(A))^{-1}
\end{equation}
It is convenient to transform to a new basis, by defining $\kappa, \gamma_1, \gamma_2$:
\begin{equation}
    \kappa=\frac{1}{2}(\psi_{11}+\psi_{22})
\end{equation}
\begin{equation}
    \gamma_1=\frac{1}{2}(\psi_{11}-\psi_{22})=\gamma\cos(2\phi(\theta))
\end{equation}
\begin{equation}
    \gamma_2=\psi_{12}=\psi_{21} = \gamma\sin(2\phi(\theta))
\end{equation}
Clearly:
\begin{equation}
    \gamma^2 = \gamma_1^2+\gamma_2^2
\end{equation}
Here, $\kappa$ is the convergence (which is directly related to the mass density), $\vec{\gamma}$ is the shear (the amount of ``stretch" of an image), and $\phi(\theta)$ is the orientation of the shear.

Thus, $A$ can be rewritten as:
\begin{equation}
    A = \begin{pmatrix}
    1-\kappa-\gamma_1 & -\gamma_2 \\
    -\gamma_2 & 1-\kappa+\gamma_1 
    \end{pmatrix}
\end{equation}
and the magnification becomes:
\begin{equation}
    {\mu=\frac{1}{[(1-\kappa)^2-\gamma^2]}}
\end{equation}

\subsection{Mass Sheet Transformation (MST)}

Lens modeling contains a degeneracy that preserves all observable except the time delay, caused by the mass sheet degeneracy.  Below, I describe this transformation.

Starting from the lens equations, we can arbitrarily multiply the equation by a constant $\lambda$: 
\begin{equation}
    \lambda\vec{\beta} = \lambda\vec{\theta} - \lambda\vec{\alpha}
\end{equation}
If we keep the observable $\vec{\theta}$ (angular separation between the lensed source and the lens) the same, we can rewrite the above equation as:
\begin{equation}
    {\vec{\beta}' = \vec{\theta} - \vec{\alpha}'}
\end{equation}
where:
\begin{equation}
    {\vec{\beta}' = \lambda\vec{\beta}} 
\end{equation}
\begin{equation}
    {\vec{\alpha}' = (1-\lambda)\vec{\theta}+\lambda\vec{\alpha}}
\end{equation}
The primed parameters are the new source position and deflection angle under this transformation defined by $\lambda$. Using equation 1.3, we can now calculate the new 2D lensing potential.
\begin{equation}
    \vec{\alpha}'(\vec{\theta})=\nabla_\theta \psi'(\vec{\theta})=(1-\lambda)\vec{\theta}+\lambda\vec{\alpha}(\vec{\theta})
\end{equation}
\begin{equation}
    \psi'(\vec{\theta}) = \frac{1-\lambda}{2}{\theta}^2+\lambda\psi(\vec{\theta})+C,
\end{equation}
The first term in the above equation represents a constant-density mass sheet (hence the name ``mass sheet transformation").  The second term is simply the scaled original 2D lensing potential.  Finally, the last term is the integration constant.  The parameter $\lambda>0$ needs to be positive for the transformed potential to have the same sign as the original potential.  One may initially think that $\lambda<1$ so that the lensing potential from the mass sheet is positive.  However, it is possible for $\lambda>1$, so long as the final mass profile (the mass sheet and the scaled original profile) is positive.  Nevertheless, in this thesis, I will assume $\lambda<1$, or $0<\lambda<1$.  The analysis can easily be generalized to $\lambda>1$.

Using the time delay formula (equation 1.4), we can calculate the effect that this transformation has on the time delay:
\begin{equation}
    \Delta t'(\vec{\theta}) = \frac{1+z_d}{c}\dTD'\left[\frac{1}{2}(\vec{\theta}-\vec{\beta}')^2-\psi'(\vec{\theta})\right]
\end{equation}
\begin{equation}
    \Delta t'(\vec{\theta}) = \frac{1+z_d}{c}\dTD'\left(\frac{\lambda}{2}{\theta}^2 - \lambda\vec{\beta}\cdot\vec{\theta} +\frac{1}{2}\lambda^2\vec{\beta}^2-\lambda\psi(\vec{\theta})-C\right)
\end{equation}

With the gauge choice of $C=\frac{\lambda^2-\lambda}{2}\vec{\beta}^2$ (\_\_\_):
\begin{equation}
    \Delta t'(\vec{\theta}) = \frac{1+z_d}{c}\dTD'\lambda\left[\frac{1}{2}(\vec{\theta}-\vec{\beta})^2-\psi(\vec{\theta})\right]
\end{equation}
Recall that only the relative time delay between two lensed images is observed.  In the presence and absence of a mass sheet, for the model-predicted relative time delays to agree with the observed value between two lensed images:
\begin{equation}
    {\dTD = \lambda\dTD'}
\end{equation}
Since the time delay distance is linearly related to $\frac{1}{H_0}$: 
\begin{equation}
    {H_0 = \frac{1}{\lambda}H'_{0}}
\end{equation}

That is, even for a very precise measurement of the relative time delay for a lensing system, $H_0$ would still have an uncertainty of $(1-\lambda)$, due to the mass sheet degeneracy. 

Repeating the magnification calculation (equations 1.6 to 1.13) for the system with MST yields:
\begin{equation}
    {\kappa'=1-\lambda+\lambda\kappa}
\end{equation}
\begin{equation}
    { \vec{\gamma}'=\lambda\vec{\gamma}}
\end{equation}
Clearly, the orientation of the shear is preserved ($\phi'=\phi$), but the magnification changes by a factor of $\frac{1}{\lambda^2}$:
\begin{equation}
    {\mu'=\frac{1}{\lambda^2}\mu}
\end{equation}

While adding a mass sheet to a lensing system is unphysical, this transformation can be approximately physically realized by varying the lensing galaxy mass profile. \_\_\_ shows that this introduces a 10\% systematic uncertainty on $H_0$ measurements based on lensed quasars, which is comparable to and therefore cannot address the Hubble tension.  Below we will show that a lensed SN Ia can significantly reduce the uncertainty from the mass sheet degeneracy.

\section{Significance of Lensed Type Ia Supernovae} \label{sec:sne1a appendix}

A SNe Ia is a type of supernova that occurs when a white dwarf (through accretion or a merging event) collapses due to its own gravity.  Once the mass of the white dwarf exceeds $\sim$1.4 solar masses (the Chandrasekhar limit), the core of the white dwarf overcomes the electron degeneracy pressure, causing an implosion followed by an explosion.  A series of nuclear fusions ensue, ending in Ni-56 with a half life of 6.1 days which powers the supernova light curve. Type Ia supernovae have standardizable peak magnitudes based on light curve shape (\citealp{e6}) and color (\citealp{tripp}).  In this thesis, I will use the SALT2 model (\citealp{e11}), which can standardize SNe Ia to $0.15$ magnitude, or about 7\% in distance measurement.  In the near future, with the twinning technique (\citealp{e7}, \citealp{boone}), the distance to SNe Ia can be measured to 3\%.  % we can use the SALT2 model to calculate the absolute magnitude of a Type Ia supernova to $\pm 0.12$ magnitude, or about $\pm 11.1\%$ flux (\cite{e11}). %Because this occurs once the white dwarf reaches the Chandrasekhar limit, Type Ia supernovae have standardizable peak magnitudes based on  approximately the same amount of nuclear fuel as well as a predictable light curve (\citealp{e6}).  With the twinning technique (\citealp{e7}), we can use the SALT2 model to calculate the absolute magnitude of a Type Ia supernova to $\pm 0.12$ magnitude, or about $\pm 11.1\%$ flux (\cite{e11}).

From equation \_\_\_, we see that the magnification $\mu$ is proportional to the squared inverse of $\lambda$.  Since supernova flux is proportional to the squared inverse of distance $D_s$:
% \begin{equation}
%     F \propto \mu \ \ , \ \  \mu \propto \lambda^{-2} \ \ , \ \  F \propto d^{-2}
% \end{equation}
\begin{equation}
    D_s \propto \lambda
\end{equation}
and
\begin{equation}
    \Delta D_s = \Delta \lambda,
\end{equation}
where $\Delta$ represents fractional uncertainty.  

% Using the SALT2 model, with distance uncertainty $\approx 7\%$, along with equation \_\_\_:

% \begin{equation}
%     \Delta H_0 = \Delta \lambda \approx 7\%
% \end{equation}

% Furthermore, using the twinning technique with systematic distance uncertainty $\approx 3\%$, $H_0$ can be even more accurately measured.  When measuring multiple lensed SNe Ia, the systematic uncertainty becomes a statistical uncertainty, as the MST produces systematic errors independent of each system.  And so, with $N$ lensed SNe Ia, the MST statistical uncertainty on $H_0$ will be:   
% \begin{equation}
%     {\Delta H_0 \approx \frac{3\%}{\sqrt{N}}}
% \end{equation}

% This represents a much improved accuracy compared with $H_0$ measurements using lensed quasars, with $\Delta H_0 \approx 10\%$ systematic uncertainty (\citealp{e8}).  Note that for modeling without the addition of a lensed standard candle, the MST is a systematic error, whereas with a lensed SN Ia (or any standard candle), the MST becomes a statistical error.  Therefore, $H_0$ measurements from lensed SNe Ia can potentially resolve the Hubble tension.%, if we are able to make use of lensed Type Ia supernovae, we can better constrain the mass sheet parameter $\lambda$, and therefore also $H_0$.  
